# Supplementary material for: ChainStream: An LLM-based Framework for Unified Synthetic Sensing
Source: arXiv:2412.15240 source file (2024-12-13)
Supplement: Supplementary file 1 [file S10_appendix.tex]

\clearpage

\begin{appendices}
% \appendix
\section{Agent Examples}
show more agent examples.

\section{Formally API Definition}
show more formal API definition, mainly for the \texttt{stream.batch()} and \texttt{llm.make\_prompt()}

% \lstinline[stye = python]|print("hello world")|
\begin{lstlisting}[style=python]
import chainstream as cs

# Agent
class Agent(cs.agent.Agent):
  def __init__(self):
    super(agent_id: str)
  def start(self):
    pass
  def stop(self):
    pass
  
# Stream
cs.stream.get_stream(
  agent: cs.agent.Agent, 
  stream_id: str
) -> cs.stream.Stream
cs.stream.create_stream(
  agent: cs.agent.Agent, 
  stream_id: str, 
  description: cs.stream.Description
) -> cs.stream.Stream
cs.stream.Stream.for_each(
  listener_func: Callable[[Union[Dict, str]], Optional[Dict]], 
  to_stream: chainstream.stream.Stream = None
) -> chainstream.stream.Stream
cs.stream.Stream.batch(
  by_count: int = None, 
  by_time: int = None, 
  by_item: Union[Dict, str] = None, 
  by_func: Callable[[Union[Dict, str], Dict], Tuple[Optional[Dict], Dict]] = None, 
  to_stream: chainstream.stream.Stream = None
) -> chainstream.stream.Stream
cs.stream.Stream.unregister_all(
  agent: cs.agent.Agent
) -> None
cs.stream.Stream.add_item(
  item: Union[Dict, str, List]
) -> None

# Buffer
cs.context.Buffer.append(
  data: Union[Dict, str]
) -> None
cs.context.Buffer.pop() -> Union[Dict, str]
cs.context.Buffer.pop_all() -> List[Union[Dict, str]]
cs.context.Buffer.get(idx) -> Union[Dict, str]
cs.context.Buffer.get_all() -> List[Union[Dict, str]]

# Model
cs.llm.get_model(
  model_type:List[Union[Literal["text", "image", "audio"]]]
) -> chainstream.llm.LLM
cs.llm.make_prompt(
  Union[Literal['str'], dict, cs.context.Buffer]
) -> str
cs.llm.LLM.query(prompt) -> str

\end{lstlisting}

\section{\generator Prompt}
show all the prompts used in the generator.

\section{Sandbox Report}
show the report details of the sandbox. \jiacheng{this section maybe not necessary}

\section{Benchmark: Tasks}
show all the tasks in the benchmark.

\section{Benchmark: Metrics}
show all the metrics in the benchmark.

\end{appendices}
